# Supplementary material for: Generative Slate Recommendation with Reinforcement Learning
Source: arXiv:2301.08632 source file (2023-01-24)
Supplement: Supplementary file 1 [file 8-appendix.tex]

\section{Appendix: Soft Actor-Critic (SAC)}
\appendix
\label{appendix}

\header{Actor-critic algorithm} In SAC, the Q-function is embodied as a critic network, i.e., a parametric function $Q_\psi : \mathcal{S} \times \mathcal{A} \rightarrow \mathbb{R}$. $Q_\psi$ is trained in an off-policy fashion to approximate the true Q-function of the current policy $\pi_{\xi}$. The critic is updated by minimizing a mean squared error loss on the temporal-difference target, i.e., one-step lookup of the current model:
\vspace{-0.05cm}
\begin{align*}
    \psi^{k+1} &= \mathrm{arg}\textstyle\min_\psi J_Q^k(\psi) \text{, with}\\[-0.1cm]  
    J_Q^k(\psi) &= \mathbb{E}_{(s,a,r,s') \sim B} \left[ \left( r + \gamma Q_{\psi^k}(s', a_{\xi^k}(s')) - Q_\psi(s, a) \right)^2 \right],
\end{align*}
where $a_{\xi^k}(s') \sim \pi_{\xi^k}(\cdot|s')$ is an action sampled from the current policy and $B$ is a buffer containing tuples of experience (state, action, reward, next state) collected earlier during the training. Then the policy (i.e., actor) is updated so as to maximize the return estimate given by the critic: 
\vspace{-0.05cm}
\begin{equation*}
    \xi^{k+1} = \mathrm{arg}\textstyle\max_\xi J_\pi^k(\xi) \,\textup{ with }
J_\pi^k(\xi) = \mathbb{E}_{s \sim B} \left[ Q_{\psi^{k+1}} \left( s, a_\xi(s) \right) \right],
\end{equation*}
where $a_\xi(s) \sim \pi_\xi(\cdot |s)$ is a sampled action. The actor-critic paradigm consists in alternating these two steps, respectively called policy evaluation and policy improvement, until convergence.
    
\header{Maximum-entropy regularization} In order to deal with the exploration-exploitation dilemma \citep{sutton-barto}, SAC adopts the maximum-entropy framework. It consists in framing the RL training as a multi-objective optimization problem between reward maximization and randomness of the policy. Concretely, the training objectives of the actor-critic model can be rewritten as follows:
\vspace{-0.05cm}
\begin{align*}
    J_Q^{k, \textup{ent}}(\psi) &=
\mathbb{E}_{(s,a,r,s') \sim B} \left[ \left( r + \gamma Q^\textup{ent}_{\psi^k, \xi^k, \alpha} (s') - Q_\psi(s, a) \right)^2 \right]\\[-0.05cm]  
    J_\pi^{k, \textup{ent}}(\xi) &= \mathbb{E}_{s \sim B} \left[ Q^\textup{ent}_{\psi^{k+1}, \xi, \alpha} (s) \right],
\end{align*}
where $Q_{\psi, \xi, \alpha}^\textup{ent} (s) = Q_{\psi} ( s, a_\xi(s) ) - \alpha \log \pi_{\xi}(a_{\xi}(s)|s)$ is the entro\-py-regularized Q-function and $ \alpha$ is a hyperparameter controlling the strength of the entropy regularization.

In this short introduction, we have omitted many implementation details such as the choice of policy parameterization, the use of clipped double Q-Learning and target networks, and automatic tuning of the entropy parameter. To learn more about SAC's implementation, we refer the reader to \citep{SAC}.
